# Supplementary material for: The compositional structure of multipartite quantum entanglement
Source: arXiv:1002.2540 source file (2010-08-17)
Supplement: Supplementary file 1 [file appendices_backup.tex]

\newpage

\appendix

%%%%%%%%%%%%%%%%%%%
%%%%%%%%%%%%%%%%%%%
\section{Proofs}\label{App:proofs}
%%%%%%%%%%%%%%%%%%%
%%%%%%%%%%%%%%%%%%%

\subsection{Proof of Theorem \ref{thm:SCFAGHZ}.}

The proof to follow is greatly assisted by this lemma.

\begin{lemma}[Mathonet et al.~\cite{Mathonet2009}]\label{thm:slocc-uniform}
	If $\ket\Psi$ and $\ket\Phi$ are symmetric $N$-qubit states such that $\ket\Psi$ and $\ket\Phi$ are SLOCC-equivalent, then there exists an invertible linear map $L:\mathbb{C}^2\to \mathbb{C}^2$ such that $\ket\Psi = L^{\otimes N} \ket\Phi$.
\end{lemma}
($\Rightarrow$; SCFA-GHZ) Let $(\mult, \unit, \comult, \counit)$ be a SCFA on $\mathbb{C}^2$ in ${\bf FHilb}$. Define another SCFA as follows:
	
		\begin{center}
			$\whitecomult :: \ket{0} \mapsto \ket{00}, \ket{1} \mapsto \ket{11}$;\qquad
			$\whitecounit := \bra{+}$;\qquad
			$\whitemult := \left( \whitecomult \right)^\dagger$;\qquad
			$\whiteunit := \left( \whitecounit \right)^\dagger$
		\end{center}
It is easy to verify that this is indeed an SCFA. It can also be verified that:
	
	\[
	\begin{tikzpicture}[dotpic,yscale=-1,yshift=5mm]
		\node [dot,fill=white] (0) at (0,-1) {};
		\node [dot,fill=white] (1) at (1,0) {};
		\node [bn] (b1) at (-2,1) {};
		\node [bn] (b2) at (0,1) {};
		\node [bn] (b3) at (2,1) {};
		\node [dot,fill=white] (b4) at (0,-2) {};
		\draw (b1)--(0)--(b4) (b2)--(1)--(b3) (0)--(1);
	\end{tikzpicture} = \lambda \ket{GHZ}
	\]
Let $\ket u, \ket v$ be the pair of linearly independent vectors copied by $\comult$. Define an invertible map $L :: \ket 0 \mapsto \ket u, \ket 1 \mapsto \ket v$. We define $\comult$ in terms of $L$ and $\whitecomult$:
	
	\[
	\comult =
	\begin{tikzpicture}[dotpic]
		\node [dot,fill=white] (0) at (0,0) {};
		\node [draw=black] (L1) at (0,1) {\footnotesize $L^{-1}$};
		\node [draw=black] (L2) at (-1,-1) {\footnotesize $L$};
		\node [draw=black] (L3) at (1,-1) {\footnotesize $L$};
		\draw (0,2)--(L1)--(0) (L2)--(-1,-2) (L3)--(1,-2);
		\draw [bend right] (0) to (L2);
		\draw [bend left] (0) to (L3);
	\end{tikzpicture}
	\]
	This induces $\unit$ as follows.
	
	\[\unit =
	\begin{tikzpicture}[dotpic]
		\node [dot] (0) at (0,0) {};
		\node [bn] (b2) at (-1,-1) {};

		\draw (0) to (b2);
		\draw (0) to [out=90,in=-90]
		    (0,1) to [out=90,in=90] 
		    (2,1) to [out=-90,in=90] 
	     (2,-1) to [out=-90,in=-90] 
			 (1,-1) to [out=90,in=-45] (0);
	\end{tikzpicture} =
	\begin{tikzpicture}[dotpic]
		\node [dot,fill=white] (0) at (0,0) {};
		\node [draw=black] (L1) at (0,1) {\footnotesize $L^{-1}$};
		\node [draw=black] (L2) at (-1,-1) {\footnotesize $L$};
		\node [draw=black] (L3) at (1,-1) {\footnotesize $L$};
		\draw (L1)--(0) (L2)--(-1,-2);
		\draw [bend right] (0) to (L2);
		\draw [bend left] (0) to (L3);
		\draw (L1) to [out=90,in=90] (2,1.6) to [out=-90,in=90] (2,-1.6) to [out=-90,in=-90] (L3);
	\end{tikzpicture} =
	\begin{tikzpicture}[dotpic]
		\node [dot,fill=white] (0) at (0,0) {};
		\node [draw=black] (L1) at (-1,-1) {\footnotesize $L$};
		
		\draw [bend right] (0) to (L1);
		\draw (L1) -- (-1,-2);
		\draw (0) to [out=90,in=-90]
		    (0,1) to [out=90,in=90] 
		    (2,1) to [out=-90,in=90] 
	     (2,-1) to [out=-90,in=-90] 
			 (1,-1) to [out=90,in=-45] (0);
	\end{tikzpicture} =
	\begin{tikzpicture}[dotpic]
		\node [dot,fill=white] (0) at (0,1) {};
		\node [draw=black] (L1) at (0,0) {\footnotesize $L$};
		\draw (0)--(L1)--(0,-1);
	\end{tikzpicture}
	\]
	It then follows that
	
	\[
	  \begin{tikzpicture}[dotpic,yscale=-1,yshift=5mm]
			\node [dot] (0) at (0,-1) {};
			\node [dot] (1) at (1,0) {};
			\node [bn] (b1) at (-2,1) {};
			\node [bn] (b2) at (0,1) {};
			\node [bn] (b3) at (2,1) {};
			\node [dot] (b4) at (0,-2) {};
			\draw (b1)--(0)--(b4) (b2)--(1)--(b3) (0)--(1);
		\end{tikzpicture} =
		\begin{tikzpicture}[dotpic,yscale=-1,yshift=5mm]
			\node [dot,fill=white] (0) at (0,-1) {};
			\node [dot,fill=white] (1) at (1,0) {};
			\node [draw=black] (b1) at (-2,1) {\footnotesize $L$};
			\node [draw=black] (b2) at (0,1) {\footnotesize $L$};
			\node [draw=black] (b3) at (2,1) {\footnotesize $L$};
			\node [dot,fill=white] (b4) at (0,-2) {};
			\draw (-2,2)--(b1)--(0)--(b4) (0,2)--(b2)--(1)--(b3)--(2,2) (0)--(1);
		\end{tikzpicture} = \lambda (L \otimes L \otimes L) \ket{GHZ}
	\]
	
\par\bigskip\noindent	($\Leftarrow$; SCFA-GHZ) In the other direction, we start with a symmetric state $\ket\Psi$ that is SLOCC with $\ket{GHZ}$. By Lemma \ref{thm:slocc-uniform}, we know $\ket\Psi$ must be of the following form, for $L$ invertible.

	\begin{equation}\label{eqn:slocc-ghz-form}
		\ket\Psi := (L \otimes L \otimes L)\ket{GHZ}
	\end{equation}
Let $\epsilon := \bra{+} L^{-1}$. Let $\textit{cap} := (\epsilon \otimes 1 \otimes 1) \circ \ket\Psi$. Now, pick a unique $\textit{cup}$ such that $\textit{cup}$ and $\textit{cap}$ form a compact structure. We can then define a SCFA as follows:
	\begin{eqnarray*}
		\whitecomult & := & \left(\textit{cup} \otimes 1 \otimes 1 \right) \circ
		              \left(1 \otimes \ket\Psi \right) \\
		\whitecounit\, & := & \bra{+} L^{-1} \\
		\whitemult& := & \left(1 \otimes \textit{cup} \right) \circ
		           \left(1 \otimes 1 \otimes \textit{cup} \otimes 1\right) \circ
		           \left(\ket\Psi \otimes 1 \otimes 1\right) \\
		\whiteunit\, & := & \left(1 \otimes \epsilon\right) \circ \textit{cap}
	\end{eqnarray*}
Taking $\ket\Psi$ to be of the form of Eq (\ref{eqn:slocc-ghz-form}), we obtain the following values:
	\begin{eqnarray*}
		\textit{cap} & := & (L \otimes L)(\ket{00} + \ket{11}) \\
		\textit{cup} & := & (\bra{00} + \bra{11})(L^{-1} \otimes L^{-1}) \\
		\whitecomult & := & (L \otimes L)(\ket{00}\bra{0} + \ket{11}\bra{1})L^-1 \\
		\whitecounit\, & := & \bra{+} L^{-1} \\
		\whitemult & := & L(\ket{0}\bra{00} + \ket{1}\bra{11})(L^{-1} \otimes L^{-1}) \\
		\whiteunit\, & := & L \ket{+}
	\end{eqnarray*}
This set of generators does indeed obey the axioms of an SCFA.

\par\bigskip\noindent ($\Rightarrow$; ACFA-W) Let	$(\mult, \unit, \comult, \counit)$ be a ACFA on $\mathbb{C}^2$ in ${\bf FHilb}$. Since $\comult$ is left and right unital, it is not separable i.e. it cannot be expressed as one of these forms: $\ket{A}\bra{b}$, $\ket{a} \otimes L$, $L \otimes \ket{a}$. 	Note that  $\lolli = tr_R(\comult)$, the result of tracing the input to the right leg. Assume without loss of generality that $\lolli$ is normal, which can be achieved by rescaling $\comult$ with some scalar $\lambda$. To avoid confusion we denote these recalled variants of $\comult$ and $\lolli$ as $\delta$ and $\ket t$. Let $B:= \left\{ \ket t, \ket{t^\perp} \right\}$ be an orthonormal basis for $\mathbb C^2$. By Prop \ref{prop:acfa-copy} we have $\delta \ket t = a \ket{tt}$. So, for some $\ket\Psi$:
	\[ \delta = a \ket{tt}\bra{t} + \ket{\Psi}\bra{t^\perp} \] 
Take the right partial trace of both sides:
	\[ \ket t = a \ket t + tr_R(\ket\Psi \bra{t^\perp}) \]
So, $tr_R(\ket\Psi \bra{t^\perp}) = (1-a)\ket t$. We can express $\ket\Psi$ in the basis $B$:
	\[ \ket\Psi = \ket{ut} + \ket{vt^\perp} \]
and
	\[ (1-a)\ket t = tr_R(\ket\Psi \bra{t^\perp}) = \ket{v} \]
Now, letting $\ket u = b\ket t + c\ket{t^\perp}$,
	\[ \ket\Psi = b \ket{tt} + c \ket{t^\perp t} + (1-a)\ket{tt^\perp} \]
Plugging in to $\delta$, letting $d = (1-a)$:
	\[ \delta = a \ket{tt}\bra{t} + \left( b\ket{tt} + c \ket{t^\perp t} + d \ket{t t^\perp} \right) \bra{t^\perp} \]
$d \neq 0$, otherwise $\delta$ is separable. Let $\ket s = \frac{1}{d}(b \ket{t} + c\ket{t^\perp})$: 
	\[ \delta = a \ket{tt}\bra{t} + \left( d \ket{st} + d \ket{t t^\perp} \right) \bra{t^\perp} \]
Note that $\ket s \neq k \ket t$, otherwise $\delta$ is separable. Also, by definition of Frobenius algebra, $\delta \eta$ is non-degenerate (i.e. entangled). So, choose non-proportional $\ket{s'}, \ket{t'}$ such that:
	\[ (\bra t \otimes 1)\delta \eta = \frac{1}{a} \ket{s'}\ \ \ \ \ \ \ (\bra{t^\perp} \otimes 1)\delta \eta = \frac{1}{d} \ket{t'}\]
Then, the state associated with $(\delta, \eta)$ is:
	\[
	  \begin{tikzpicture}[dotpic,xscale=-1,yscale=-1,yshift=5mm]
			\node [dot] (0) at (0,-1) {};
			\node [dot] (1) at (1,0) {};
			\node [bn] (b1) at (-2,1) {};
			\node [bn] (b2) at (0,1) {};
			\node [bn] (b3) at (2,1) {};
			\node [dot] (b4) at (0,-2) {};
			\draw (b1)--(0)--(b4) (b2)--(1)--(b3) (0)--(1);
		\end{tikzpicture} =\lambda 
	(\delta \otimes 1) \delta \eta = \lambda(\ket{tts'} + \ket{stt'} + \ket{tt^\perp t'}) \]
Now, define the following local maps:
	\[ L_1 ::  \ket t \mapsto \ket 0, \ket s \mapsto \ket 1  \]
	\[ L_2 ::  \ket t \mapsto \ket 0, \ket{t^\perp} \mapsto \ket 1  \]
	\[ L_3 ::  \ket{t'} \mapsto \ket 0, \ket{s'} \mapsto \ket 1 \]
These are all invertible because they take bases to bases. Then
	\[ (L_1 \otimes L_2 \otimes L_3)(\delta \otimes 1) \delta \eta = \ket{W} \]


\par\bigskip\noindent ($\Leftarrow$; ACFA-W) For the converse, we mirror the construction from the proof of the SCFA-GHZ case. The only difference is the choice of counit. Start with a symmetric state $\ket\Psi$ that is SLOCC with $\ket W$. By Lemma \ref{thm:slocc-uniform}, we know $\ket\Psi$ must be of the following form, for $L$ invertible.
\begin{equation}\label{eqn:slocc-w-form}
	\ket\Psi := (L \otimes L \otimes L)\ket{W}
\end{equation}
Let $\epsilon := \bra{0} L^{-1}$. Let $\textit{cap} := (\epsilon \otimes 1 \otimes 1) \circ \ket\Psi$. Now, pick a unique $\textit{cup}$ such that $\textit{cup}$ and $\textit{cap}$ form a compact structure. We can then define an ACFA as follows:
\begin{eqnarray*}
	\comult & := & \left(\textit{cup} \otimes 1 \otimes 1 \right) \circ
	              \left(1 \otimes \ket\Psi \right) \\
	\counit\, & := & \bra{0} L^{-1} \\
	\mult & := & \left(1 \otimes \textit{cup} \right) \circ
	           \left(1 \otimes 1 \otimes \textit{cup} \otimes 1\right) \circ
	           \left(\ket\Psi \otimes 1 \otimes 1\right) \\
	\unit\, & := & \left(1 \otimes \epsilon\right) \circ \textit{cap}
\end{eqnarray*}
Taking $\ket\Psi$ to be of the form of Eq (\ref{eqn:slocc-w-form}), we obtain the following values:
\begin{eqnarray*}
	\textit{cap} & := & (L \otimes L)(\ket{10} + \ket{01}) \\
	\textit{cup} & := & (\bra{10} + \bra{01})(L^{-1} \otimes L^{-1}) \\
	\comult & := & (L \otimes L)(\ket{10}\bra{1} + \ket{01}\bra{1} + \ket{00}\bra{0})L^-1 \\
	\counit\, & := & \bra{0} L^{-1} \\
	\mult & := & L(\ket{1}\bra{11} + \ket{0}\bra{01} + \ket{0}\bra{10})(L^{-1} \otimes L^{-1}) \\
	\unit\, & := & L \ket{1}
\end{eqnarray*}
This set of generators does indeed obey the axioms of an ACFA.

\subsection{Proof of Corollary  \ref{cor:cfa-local-equiv}.}
	Each CFA on $\mathbb{C}^2$ in ${\bf FHilb}$ induces a tripartite qubit state $S_3^0 = \threestate$, which, as a consequence of the CFA being unital, is non-degenerate.  Hence it either must be SLOCC-equivalent to $\ket{GHZ}$ or $\ket{W}$, so we can apply the construction in the proof of Thm \ref{thm:SCFAGHZ}. This preserves $\threestate$, yet yields a new cup:
	\begin{tikzpicture}[dotpic,scale=0.5,yscale=-1]
		\draw (0,-0.5) to [out=90,in=180] (1,0.5) to [out=0,in=90] (2,-0.5);
		\node [white dot,inner sep=0pt] (0) at (1,0.5) {$\cdot$};
	\end{tikzpicture}. Let $L$ from the corollary then be the composition of the old cap with the new cup.
	\[
	\begin{tikzpicture}[dotpic]
		\node [square box,fill=none,inner sep=0pt] (0) at (0,0) {\small L};
		\draw (0,1)--(0)--(0,-1);
	\end{tikzpicture} =
	\begin{tikzpicture}[dotpic,yshift=-5mm,scale=0.5]
			\node [bn] (b0) at (-1,2) {};
			\node [white dot,inner sep=0pt] (0) at (0,0) {$\cdot$};
			\node [dot] (1) at (1.5,1) {};
			\node [bn] (b1) at (2.5,-1) {};
			\draw (b0) to [out=-90,in=180] (0) (0) to [out=0,in=180] (1) (1) to [out=0,in=90] (b1);
		\end{tikzpicture}
	\]

\subsection{Proof of Corollary \ref{cor:2d-frobenius-form}.}
	We begin by recalling an equivalent definition of a Frobenius algebra (see e.g. \cite{KockApp}), spelled out for the specific case of ${\bf FHilb}$.
	
	\begin{definition}\label{def:std-frobenius}\em 
		A \em Frobenius algebra over $\mathbb C$ \em is a monoid $(A, \mu, \eta)$ with a linear functional $\epsilon : A \rightarrow \mathbb C$ such that $\epsilon\mu$ is a \em non-degenerate pairing\em. That is, the induced map:
		\[ \widehat{\epsilon\mu} :: u \mapsto \epsilon\mu(1 \otimes u) \]
		is invertible. In such a case, $\epsilon$ is called a \em Frobenius form\em.
	\end{definition}
	
	Since $\epsilon$ fixes an isomorphism with the dual space, it uniquely determines a comultiplication $\delta$, from which we can recover the definition of Frobenius algebra given in section \ref{sec:Frob}.
	
	Let $(A, \mu, \eta)$ be a (commutative) monoid. $\mu$ is unital, so in particular, must be connected.
	 Therefore, using \cite{DVCApp}, for $M$ one of the following:
	\[
	M = \mu_{GHZ} = \ket{0}\bra{00} + \ket{1}\bra{11}
	\qquad\textit{or}\qquad
	M = \mu_{W} = \ket{0}\bra{00} + \ket{1}(\bra{10} + \bra{01})
	\]
we have $\mu = (L_1) M (L_2 \otimes L_3)$, for some invertible maps $L_i$. In the case where $M = \mu_{GHZ}$, let $\epsilon = \bra + (L_1^\inv)$. Then $\epsilon\mu = (\bra{00} + \bra{11})(L_2 \otimes L_3)$. For $L_i$ invertible, $\epsilon\mu$ is a non-degenerate pairing. In the case where $M = \mu_{W}$, let $\epsilon = \bra 1 (L_1^\inv)$. Then $\epsilon\mu = (\bra{10} + \bra{01})(L_2 \otimes L_3)$, which is also a non-degenerate pairing. It then follows that $(A, \mu, \eta)$ extends to a Frobenius algebra. Furthermore, if $\mu$ is commutative, $\epsilon\mu$ is symmetric and the induced FA is also commutative.

%%%%%%%%%%%%%%%%%%%
%%%%%%%%%%%%%%%%%%%
\section{Classical multiplexers versus QMUX}\label{App:QMUX}
%%%%%%%%%%%%%%%%%%%
%%%%%%%%%%%%%%%%%%%

The classical multiplexer (MUX) is a device that acts as a two-way switch. An input of 0 on the control line connects the first input to the output, and an input of 1 connects the second. It is often represented schematically as follows:
\begin{center}
	\includegraphics[scale=1]{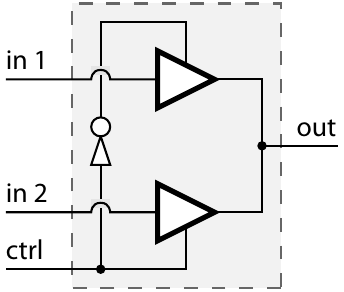}
\end{center}
The logic gate that does the critical work of the MUX is the 3-state gate, or tristate, which behaves as an electronic switch, with the side input taking a control bit.
\begin{center}
	\includegraphics[scale=1]{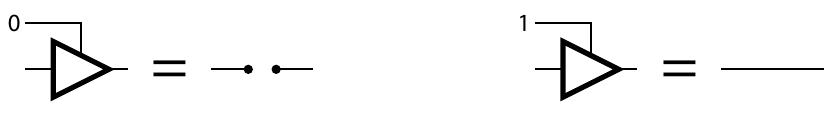}
\end{center}

This looks very similar, topologically, to the behaviour of the multiplication for an ACFA . Let $\unit$ and $\lolli$ be the two possible inputs for the control qubit, then:
\begin{center}
	\begin{tikzpicture}[dotpic]
		\node [bn] (b0) at (0,1) {};
		\node [dot] (0) at (0,0) {};
		\node [dot] (1) at (-0.7,0.7) {};
		\node [bn] (b1) at (0,-1) {};
		\draw [uploop] (1) to ();
		\draw [bend right] (1) to (0);
		\draw (b0)--(0)--(b1);
	\end{tikzpicture}\ \ = 
	\begin{tikzpicture}[dotpic]
		\node [bn] (0) at (0,1.3) {};
		\node [dot] (1) at (0,0.7) {};
		\node [dot] (2) at (0,-0.7) {};
		\node [bn] (3) at (0,-1.3) {};
		\draw (0)--(1) (2)--(3);
		\draw [downloop] (1) to ();
		\draw [uploop] (2) to ();
	\end{tikzpicture}
	\qquad\qquad
	\begin{tikzpicture}[dotpic]
		\node [bn] (b0) at (0,1) {};
		\node [dot] (0) at (0,0) {};
		\node [dot] (1) at (-0.7,0.7) {};
		\node [bn] (b1) at (0,-1) {};
		\draw [bend right] (1) to (0);
		\draw (b0)--(0)--(b1);
	\end{tikzpicture}\ \ = 
	\begin{tikzpicture}[dotpic]
		\node [bn] (0) at (0,1.3) {};
		\node [bn] (3) at (0,-1.3) {};
		\draw (0)--(3);
	\end{tikzpicture}
\end{center}

Using this intuition, let us pretend (roughly) that SCFA dots acts as junctions, ACFA dots act as tristates and the tick acts as a NOT gate. We get a ``quantumised'' diagram that is very similar to the classical one.

\begin{center}
	\raisebox{-36pt}{\includegraphics[scale=1]{mux.pdf}}
	\qquad {\Huge $\Rightarrow$} \qquad
	\raisebox{-36pt}{\includegraphics[scale=1]{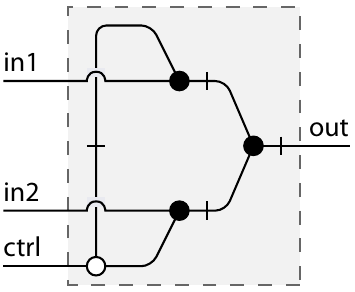}}
\end{center}

For our purposes, we would like to have the control line on an output, so doing a bit of manipulation, we get a more convenient form.
\begin{equation*}
	\raisebox{-20pt}{\includegraphics[scale=0.7]{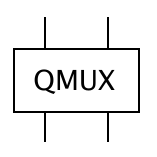}}
	:=
	\begin{tikzpicture}[dotpic,yshift=0.5cm]
		\node [bn] (d1) at (0,0.7) {};
		\node [bn] (d2) at (1,0.7) {};
		\node [dot] (0) at (0,0) {};
		\node [dot] (1) at (1,0) {};
		\node [white dot] (2) at (0,-1) {};
		\node [dot] (3) at (1,-1) {};
		\node [bn] (c1) at (0,-1.7) {};
		\node [bn] (c2) at (1,-1.7) {};
		\draw
			(d1)--(0)-- node[tick]{-} (2)-- node[tick]{-} (c1)
			(d2)--(1)-- node[tick]{-} (3)-- node[tick]{-} (c2)
			(0)-- node[tick,pos=0.7]{-} (3)  (1)--(2);
	\end{tikzpicture}
\end{equation*}

This provides a quantum analogue to the classical multiplexor. However, rather than impeding (i.e. ``disconnecting'') the unwanted line, linearity forces us to project it out. Luckily, when considering inputs and/or outputs only up to SLOCC, this oddity can often be rectified.

%%%%%%%%%%%%%%%%%%%
%%%%%%%%%%%%%%%%%%%
\section{Symmetric monoidal categories and graphical calculus.}\label{App:SMC}
%%%%%%%%%%%%%%%%%%%
%%%%%%%%%%%%%%%%%%%

In categories where objects admit a tensor product, such as ${\bf FHilb}$, the category of finite-dimensional complex Hilbert spaces and linear maps, $\otimes$ is a monoid on objects \emph{up to isomorphism},  with the underlying field $\mathbb{C}$ as its unit.  This monoid structure on objects  extends in a natural way to a bifunctor. 

A \em monoidal category \em is a category ${\bf C}$, with a bifunctor 
\[
(- \otimes -) : {\bf C} \times {\bf C} \rightarrow {\bf C}
\]
 that is (weakly) associative and unital. Weak associativity means there exists a natural isomorphism $\alpha$ such that for all objects $A,B,C \in {\bf C}$,
\[ \alpha_{A,B,C} : (A \otimes B) \otimes C \cong A \otimes (B \otimes C).\]

Weak unity means there exists an object $I$ and two natural isomorphisms $\lambda$ and $\rho$ such that $\lambda_A : A \cong I \otimes A$ and $\rho_A: A \cong A \otimes I$. These isomorphisms are subject to certain coherence properties (see e.g.~\cite{MacLane}).

A \emph{strict monoidal functor} $F : \mathcal C \rightarrow \mathcal D$ between monoidal categories is a functor that preserves the monoidal product: $F(A \otimes B) = FA \otimes FB$. A \emph{strict monoidal natural transformation} $\mu$ is a natural transformation such that $\mu_{A\otimes B} = \mu_A \otimes \mu_B$.

In many monoidal categories, the two objects $A \otimes B$ and $B \otimes A$ are isomorphic. If there is a \textit{natural} isomorphism $\sigma_{A,B} : A \otimes B \cong B \otimes A$ that interacts in a sensible way with $\otimes$ and $\alpha$, i.e. this equation holds:
\[
(1_B \otimes \sigma_{A,C}) \circ \alpha_{B,A,C} \circ (\sigma_{A,B} \otimes 1_C) =
(\alpha_{B,C,A} \circ (\sigma_{B,C\otimes A}) \circ \alpha_{A,B,C}
\]
then $\sigma$ is called a \emph{braiding}, and ${\bf C}$ a \emph{braided monoidal category}. If furthermore, $\sigma_{A,B} \circ \sigma_{A,B} = 1_{A\otimes B}$, then $\sigma$ is called a symmetry, and ${\bf C}$ is a \emph{symmetric monoidal category}.
A braided (resp. symmetric) monoidal functor is just a monoidal functor that preserves braidings (resp. symmetries).

There are many examples of symmetric monoidal categories. Our main example will be ${\bf FHilb}$. For any two Hilbert spaces $A$ and $B$, there is a symmetry
\[
\sigma_{A,B} : A \otimes B \rightarrow B \otimes A :: \psi \otimes \phi \mapsto \phi \otimes \psi
\]
Since the tensor unit in ${\bf FHilb}$ is $\mathbb C$, we note that a linear map $s:\mathbb C\to \mathbb C$ can be identified by the  scalar $s(1)\in\mathbb C$. We extend this to a general notion.
More general, in a monoidal category $({\bf C}, \otimes, I)$, any map $f : I \rightarrow I$ is called a \textit{scalar}.

Another important structure in ${\bf FHilb}$ we wish to capture is the property of having a dual space. We say $A$ \emph{has a dual} if there exists an object $A^*$ and maps $d_A: I \rightarrow A^* \otimes A$ and $e_A : A \otimes A^* \rightarrow I$ such that

\begin{equation}\label{eq:has-dual}
	(1_A \otimes d_A) \circ (e_A \otimes 1_A) = 1_A\qquad
	(d_A \otimes 1_A) \circ (1_A \otimes e_A) = 1_{A^*}
\end{equation}

A symmetric monoidal category is \emph{compact closed} if all objects have duals.	When we fix an object $A$, its dual is only determined up to isomorphism. Therefore, when $A$ is isomorphic with its dual, as is always the case in finite-dimensional Hilbert spaces, we can choose the \textit{categorical} dual to be $A$ itself. In such a situation, we say $A$ is \textit{self dual}.  For example, objects which come with a commutative Frobenius algebra (see Section \ref{sec:Frob}) always are self-dual.


Again these maps have to interact coherently with the other elements of the symmetric monoidal structure. For an explicit statement of these coherence properties, see \cite{SelingerSurveyApp}. We avoid the verbose technical definition here, but we will still make an exact definition of coherence shortly, by introducing the graphical notation for compact closed categories.

\subsection{Graphical representation}\label{sub:graphical-rep}

The theory of monoidal categories is in a strong sense a 2-dimensional theory. One interpretation for this dimensionality is that the tensor product provides a spacial dimension, while the composition of arrows provides temporal, or causal dimension. The interplay of these two dimensions is represented by the bifunctoriality of the tensor product.
\begin{equation}\label{eq:bifunc}
	(f_2 \otimes g_2) \circ (f_1 \otimes g_1) = (f_2 \circ f_1) \otimes (g_2 \circ g_1)
\end{equation}

One can interpret this equation by thinking of these four arrows occupying a piece of 2-dimensional space.

\tikzstyle{dashed box}=[draw=black,dashed,minimum height=12mm,minimum width=12mm,fill=gray!20]
\begin{center}
	\tikzfig{2d_space}
\end{center}

From this point of view, the bracketing in Eq (\ref{eq:bifunc}) is a piece of essentially meaningless syntax, which is required to make something that is 2-dimensional by nature expressible as a (1-dimensional) term. To address this issue, we shall introduce a graphical notation for symmetric monoidal categories, similar to that of circuit diagrams. Edges represent objects and nodes represent morphisms. Normally, both edges and nodes are labeled, but here we shall consider only graphs where every edge represents the same object, so we shall omit edge labels. Tensoring is done by juxtaposition and composition is performed by \emph{plugging}, or gluing the inputs of one graph to the outputs of another. The identity arrow is represented by an empty edge and the tensor unit by an empty graph.\vspace{-1mm}
\begin{equation}\label{eqn:graphical-compose}
	\tikzfig{gluing_and_juxt}
\end{equation}
Since we can express $A \otimes A$ as a pair of lines, we can, for instance, express a map $h : A \otimes A \rightarrow A \otimes A$ and compose in various ways with other maps.\vspace{-1mm}
\begin{equation}\label{eqn:mixed-arities}
	\tikzfig{mixed_arities}
\end{equation}
We can express the bifunctoriality of $\otimes$ and the naturality of $\sigma$ as follows:\vspace{-1mm}
\begin{equation}\label{eqn:graphical-bifunc}
	\tikzfig{bifunc}
	\hspace{10mm}
	\tikzfig{symmetry_natural}
\end{equation}

Edges, nodes, and edge crossings provide a graphical language for symmetric monoidal categories. This language captures exactly the coherence properties present in a symmetric monoidal category. Selinger states this precisely in \cite{SelingerSurveyApp}.

\begin{theorem}\label{thm:smc-coherence}
	(Coherence for symmetric monoidal categories). A well-formed equation between morphisms in the language of symmetric monoidal categories follows from the axioms of symmetric monoidal categories if and only if it holds, up to isomorphism of diagrams, in the graphical language.
\end{theorem}

So far, we have introduced a graphical language for describing terms in a symmetric monoidal category. These terms are precisely the directed acyclic graphs generated by the arrows in that category. If the line represents an object $A$, and $A$ has a dual, we can actually express terms as \emph{arbitrary} graphs. We represent the type $A$ as a line directed down, $A^*$ as a line directed up, and the maps $d_A$ and $e_A$ from the previous section as caps and cups.

\begin{equation}\label{eq:graphical-compactness}
	\tikzfig{graphical_compactness}
\end{equation}

\begin{theorem}\label{thm:ccl-coherence}
	(Coherence for compact closed categories). A well-formed equation between morphisms in the language of compact closed categories follows from the axioms of compact closed categories if and only if it holds, up to isomorphism of diagrams, in the graphical language.
\end{theorem}

\subsection{Relationship with the Circuit Model}\label{App:circuit}

Anyone with some familiarity of the quantum circuit model will have seen diagrams that look like (\ref{eqn:graphical-compose}) and (\ref{eqn:mixed-arities}). This is because quantum circuit diagrams are a special case of the graphical representation of monoidal categories. Traditionally, circuit diagrams are just graphs that are \textit{planar} and \textit{directed acyclic}. These are exactly the kinds of graphs one can construct in a monoidal category if one refrains from using the symmetric, compact structure of the category. Selinger's survey \cite{SelingerSurveyApp} offers a result (originally due to Joyal and Street) about these kinds of graphs as well, for the sake of completeness.

\begin{theorem}\label{thm:planar-coherence}
	(Coherence for planar monoidal categories). A well-formed equation between morphism terms in the language of monoidal categories follows from the axioms of monoidal categories if and only if it holds, up to planar isotopy, in the graphical language.
\end{theorem}

Here, planar isotopy means simply that one graph can be deformed into another without crossing edges. Circuit diagrams also tend to run in ``tracks,'' parallel lines that clearly distinguish qubits. This rigidity comes from the fact that circuit components are unitary, so tend to have the same number of input and output wires. However, this convention is purely pedagogical, as arbitrary planar, directed acyclic graphs can be interpreted as circuits without ambiguity.

What symmetry makes explicit is the act of swapping qubits, rather than encoding it with quantum gates, such as 3 controlled-not gates:

\begin{equation}
	\begin{tikzpicture}[dotpic,yshift=1.75cm,-latex]
		\node [bn] (d1) at (0,-0.5) {};
		\node [bn] (c1) at (2,-3) {};
		\node [bn] (d2) at (2,-0.5) {};
		\node [bn] (c2) at (0,-3) {};

		\draw [rounded corners=1mm]
			(d1) -- (0,-1) -- (2,-2.5) -- (c1);
		\draw [rounded corners=1mm]
			(d2) -- (2,-1) -- (0,-2.5) -- (c2);
	\end{tikzpicture}
	:=
	\begin{tikzpicture}[dotpic,scale=2,yshift=5mm]
		\draw (0,0)--(1,0);
		\draw (0,-0.5)--(1,-0.5);
		\draw (0,-1)--(1,-1);
		\draw (0,0.3)--(0,-1.3);
		\draw (1,0.3)--(1,-1.3);
		\node [small dot] (0) at (1,0) {};
		\node [cnot] (1) at (0,0) {$\oplus$};
		\node [small dot] (0) at (0,-0.5) {};
		\node [cnot] (1) at (1,-0.5) {$\oplus$};
		\node [small dot] (0) at (1,-1) {};
		\node [cnot] (1) at (0,-1) {$\oplus$};
	\end{tikzpicture}
\end{equation}

Making this definition allows line crossings, and we can do away with the needless restriction that diagrams be planar. Compact structures can be encoded in the circuit model as well, using Bell-states and Bell-effects~\cite{ACApp}. 

\begin{thebibliography}{99}
\bibitem[a1]{ACApp}
S.~Abramsky and B.~Coecke (2004) {\em A categorical
semantics of quantum protocols}.  LiCS`04. Revision: arXiv:quant-ph/0808.1023
\bibitem[a2]{DVCApp}
W.~D\"ur, G.~Vidal and J.~I.~Cirac (2000) 
\em Three qubits can be entangled in two inequivalent ways\em.  
Phys.~Rev.~A {\bf 62}, 062314. arXiv:quant-ph/0005115
\bibitem[a3]{KockApp}
J.~Kock (2003) \em Frobenius Algebras and 2D Topological Quantum Field Theories\em. Cambridge 
\bibitem[a6]{SelingerSurveyApp}
P.~Selinger (2009) \em A survey of graphical languages for monoidal categories\em. In: New Structures for Physics, B.~Coecke (ed), 275--337, Springer-Verlag. 
arXiv:0908.3347
\end{thebibliography}

\end{document}

 
% LocalWords:  LiCS FHilb SMC SMCs wp UU BlochGreen pdf deltadag epsilondag eq
% LocalWords:  odot defn defnbis commutebis psidelta psiepsilon BlochPhase CCSs
% LocalWords:  defdiamond eigenvectorbis ij bialgebralawbis hopflawbis eqs tris
% LocalWords:  Hepsilon Hsquared Hdelta CXdefnbis CXgate CXcorrectness CXproof
% LocalWords:  CZdefn CZproofbis Shor's Cphase QFTcircuit QFTproofbis wqcCX th
% LocalWords:  clusterCZbis clusterPEPSbis clusterequiv wqcU IEEE linearizing
% LocalWords:  ENTCS POVMs aimark's Kauffman Lamonaco Vicary ACM otteler PROPs
% LocalWords:  selinger odinger rr rrrr eigen ZX XZ hopfproof CALCO practicing
% LocalWords:  Polimetrica Generalized nd Verlag Kluwer AÊ quant ph Birkhoff
% LocalWords:  factorization von Neumann Pavlovic Carboni Abramsky CCS Hopf
% LocalWords:  Klappenecker Hadamard Coecke Danos Kashefi Panangaden Joyal Kock
